# Supplementary material for: Improved Guarantees for k-means++ and k-means++ Parallel
Source: arXiv:2010.14487 source file (2020-10-27)
Supplement: Supplementary file 1 [file unused-parallel-additional-results.tex]

\section{\texorpdfstring{Additional results for $k$-means\kpp}{Additional results for k-means Parallel}}\label{apx:kpp}
In Section~\ref{sec:po-kmeans-parallel}, we gave several bounds on the expected cost of clustering produced by the $k$-means$\kpp$ algorithm. In this section, we show that, for $\ell \geq k$, the upper bound for the expected cost of clustering converges to $5\opt$ as the number of rounds $T$ increases (we get a bound of $8\opt$ from Theorem~\ref{lem:parallel_1}). More specifically, we show that the expected cost of clustering is upper bounded by $(5+O(1/T))\opt_k(\pointset)$ when $T \geq \ln(\opt_1(\pointset)/\opt_k(\pointset))$.

\begin{theorem}
Consider a data set $\pointset$ with more than $k$ distinct points. Let $T_0 = \ln(\opt_1(\pointset)/\opt_k(\pointset))$ and  $\ell \geq k$. The expected cost of the clustering returned by $k$-means$\kpp$ algorithm after $T \geq T_0$ rounds is upper bounded as follows:
$$
    \expect{\cost_{T}(\total)} \leq \rbr{ \frac{18}{\beta(T-T_0+t_0)}+ 5}\opt_k(\pointset),
$$
where $\beta = k(1-e^{-\ell/k})/\ell$ and $t_0 = \ceil{2(1-\beta)/\beta}$.
\end{theorem}

To prove this theorem, we need to define functions $F_t^\beta(x)$.
\begin{definition}~\label{def:recurrence}
Let $\{F_t^\beta(x), t \geq 0\}$ be a sequence of functions satisfying the following recurrence relation:
$$
    F_{t+1}^\beta(x) = F_t^\beta\rbr{\rbr{1-\beta\cdot\frac{x}{x+1}}x}, F_0^\beta(x) = x,
$$
where the parameter $\beta = k(1-e^{-\ell/k})/\ell$.
\end{definition}
We show that functions $\cbr{F_t^\beta}$ are concave and monotone increasing.

\begin{lemma}~\label{lem:Concave_Monotone}
The functions $\{F_t^\beta(x), t \geq 0, x \geq 0\}$ are concave and monotone increasing for all $t$.
\end{lemma}
\begin{proof}
We prove this by induction on $t$.
For base case, $F_0^\beta(x) = x, F_1^\beta(x) = \rbr{1-\beta x/(x+1)}x$ are concave and monotone increasing as:
$$
(F_1^\beta)'(x) = 1 - \beta + \frac{\beta}{(x+1)^2} > 0
$$ and
$$
(F_1^\beta)''(x) = - \frac{2\beta}{(x+1)^3} < 0.
$$
%This follows from the fact that $e^{-x} \geq 1 - x$ for any $x \in \R$.
Assume $F_k^\beta(x)$ is concave and monotone increasing for some $k \geq 0$, then $F_{k+1}^\beta(x) = F_k^\beta\rbr{F_1^\beta(x)}$.
\\By the inductive hypothesis, $F_k^\beta(x)$ is concave and monotone increasing and we know that $F_1^\beta(x)$ is concave and monotone increasing. The composition of two monotone increasing functions is monotone increasing. We also know that for any functions $f(x), g(x)$ such that $f(x)$ is concave and monotone increasing, $g(x)$ is concave, we have that $f(g(x))$ is concave. Therefore, $F_{k+1}^\beta(x)$ is concave.
\end{proof}

\begin{lemma}~\label{lem:Concave_Monotone_2}
For any constant $\alpha > 0$, the functions $G_t^\beta(x) = F_t^\beta(\alpha/ x)x$ are concave and monotone increasing for any $x > 0$.
\end{lemma}

\begin{proof}
By Lemma~\ref{lem:Concave_Monotone}, we have for $x > 0$
$$
(G_t^\beta)'(x) = F_t^\beta(\alpha / x) - \frac{\alpha}{x} (F_t^\beta)'(\alpha / x) \geq 0,
$$
and
$$
(G_t^\beta)''(x) = (F_t^\beta)''(\alpha / x) \alpha^2 /x^3 \leq 0.
$$
which means $G_t^\beta(x)$ is concave and monotone increasing on $(0,\infty)$.
\end{proof}

For small $x$, we show that $F_t^\beta(x)$ can be upper bounded by $\sfrac{2}{\beta(t+t_0)}$ for some constant $t_0$. Actually, using program to compute $F_t^\beta$, we found that $F_t^\beta(x)$ will be very close to $\sfrac{1}{\beta(t+t_0)}$ for $x \leq 1/2$.

\begin{lemma}~\label{lem:F_decay}
Let $\beta = k(1-e^{-\ell/k})/\ell$ and $t_0 = \ceil{2(1-\beta)/\beta}$. For any $x_0 \leq 2/ (\beta t_0)$ and any $t \geq 0$, we have
$$
F_t^\beta(x_0) \leq \frac{2}{\beta (t+t_0)}.
$$
\end{lemma}

\begin{proof}
Let $a_t = 1/F_t^\beta(x_0)$. By definition~\ref{def:recurrence}, we have
$$
a_{t+1} = a_t + \beta - \frac{\beta(1-\beta)}{a_t + (1-\beta)}.
$$
Then, we show that $a_t \geq \beta (t+t_0)/2$ for any $t \geq 0$ by induction. For Base case, it is obvious that $a_0 = 1/x_0 \geq \beta t_0 /2$.

Suppose $a_t \geq \beta (t+t_0)/2$, we show that $a_{t+1} \geq \beta(t+t_0+1)/2$.
Since $t_0 = \ceil{2(1-\beta)/\beta}$, we can get
$$
a_t \geq \beta(t+t_0)/2 \geq 1-\beta,
$$
Therefore,
$$
a_{t+1} \geq \frac{\beta (t+t_0)}{2} + \beta - \frac{\beta}{2} \geq \frac{\beta (t+t_0+1)}{2}.
$$
Since $F_t^\beta (x_0) = 1/a_t$, we have $F_t^\beta (x_0) \leq 2/(\beta (t+t_0))$.
\end{proof}

 Given the center set after $t$ rounds $\centerset_t$, let
 \begin{align*}
     \UU_{t+1}(\cluster_i) =
     \begin{cases}
       0, & \mbox{if $P_i$ is covered} \\
      \cost(P_i,C_t), & \mbox{otherwise}.
     \end{cases}
 \end{align*}
 denote the uncovered cost after the first stage of round $t+1$.
 Let $\widehat{H}_t(\cluster_i)$ be an upper bound of $H_t(\cluster_i)$. If $P_i$ is covered by $C_t$, then $\widehat{H}_t(P_i) = H_{t_i}(P_i)$,
where $t_i\leq t$ is the first time when $P_i$ is covered by $C_t$. If $P_i$ is not covered by $C_t$, then $\widehat{H}_t(P_i)=0$.

\begin{lemma}\label{lem:uncovered}
For $k$-means$\kpp$ algorithm with parameter $\ell$, the
 following  bounds hold,
$$
\expect{\UU_{t+1}(\pointset) \mid \centerset_t} \leq F_1^\beta\rbr{\frac{U_t (\pointset)}{\HH_t(\pointset)}}\HH_t(\pointset),
$$
where $F_1^\beta(x) = \rbr{1-\beta\frac{x}{x+1}}x$ with $\beta = k(1-e^{-\ell/k})/\ell$.
\end{lemma}

\begin{proof}
By the definition of $\UU_{t+1}$, we have
\begin{align*}
    \expect{\UU_{t+1}(\pointset) \mid \centerset_t} &= \sum_{i=1}^k \prob{Z_{t+1}(\cluster_i) = 0} U_t(\cluster_i) \leq \sum_{i=1}^k \exp\rbr{- \frac{\ell U_t(\cluster_i)}{U_t(\cluster_i)+\widehat{H}_t(\cluster_i)}} U_t(\cluster_i).
\end{align*}
Using $f(x) = e^{-x}\cdot x$, this expectation can be written as
$$
    \expect{\UU_{t+1}(\pointset) \mid \centerset_t} = \rbr{\frac{1}{k}\sum_{i=1}^k f\rbr{\frac{\ell U_t(\cluster_i)}{U_t(\cluster_i) + \widehat{H}_t(\cluster_i)}}} \frac{k(U_t(\cluster_i) + \widehat{H}_t(\cluster_i))}{\ell}.
$$
Since $f(x)$ is concave on $[0,1]$ and $f(x) < e^{-1}$ on $(1,\infty)$, the concave hull of $f(x)$ on $[0,\infty)$ is
\begin{align*}
    g(x) =
    \begin{cases}
     f(x)  &  \text{if $x \in [0,1]$,} \\
    e^{-1} &  \text{if $x \in (1,\infty)$.}
    \end{cases}
\end{align*}

By the concavity of function $g$, we can get
\begin{align*}
    \expect{\UU_{t+1}(\pointset) \mid \centerset_t}
    \leq& \rbr{\frac{1}{k} \sum_{i=1}^k g\rbr{\frac{\ell U_t(\cluster_i)}{U_t(\cluster_i) + \widehat{H}_t(\cluster_i)}}} \frac{k(U_t(\cluster_i) + \widehat{H}_t(\cluster_i))}{\ell} \\
    \leq& g\rbr{\frac{\ell U_t(\pointset)}{k (U_t(\pointset) + \widehat{H}_t(\pointset))}} \frac{k(U_t(\pointset) + \widehat{H}_t(\pointset))}{\ell}.
\end{align*}
When $\ell > k$ and $(\ell-k)U_t(\pointset) > k\widehat{H}_t(\pointset)$, we have
$$
    \expect{\UU_{t+1}(\pointset) \mid \centerset_t} \leq \rbr{\frac{k}{e\ell}} (U_t(\pointset)+\widehat{H}_t(\pointset)) \leq \frac{U_t(\pointset)}{e}.
$$
Since $(1-e^{-x})/x$ is monotone increasing on $[1,\infty)$, we have for $\ell > k$
$$
1-\frac{k(1-e^{-\ell/k})}{\ell} \geq e^{-1}.
$$
Thus, we have
\begin{align*}
    \expect{\UU_{t+1}(\pointset) \mid C_t} \leq \rbr{1-\frac{k(1-e^{-\ell/k})}{\ell}\frac{U_t(\pointset)}{U_t(\pointset)+\HH_t(\pointset)}}U_t(\pointset).
\end{align*}
Otherwise, we have
\begin{align*}
    \expect{\UU_{t+1}(\pointset) \mid \centerset_t} \leq \exp\rbr{-\frac{\ell U_t(\pointset)}{k (U_t(\pointset)+\widehat{H}_t(\pointset))}} \cdot U_t(\pointset)
    \leq \exp\rbr{-\frac{\ell U_t(\pointset)}{k (U_t(\pointset)+\HH_t(\pointset))}} \cdot U_t.
\end{align*}
Since $1-(1-e^{-\ell-k})kx/\ell \geq e^{-x}$ on $[0,\ell/k]$, we have
\begin{align*}
    \expect{\UU_{t+1}(\pointset) \mid \centerset_t} \leq \rbr{1- \frac{k\rbr{1-e^{-\ell/k}}}{\ell}\frac{U_t(\pointset)}{U_t(\pointset)+\HH_t(\pointset)}}U_t(\pointset).
\end{align*}
which concludes this lemma.
\end{proof}

Then, we provide an analysis to the expected uncovered cost after $t$ rounds in $k$-means\kpp.

\begin{lemma}\label{lem:recursive}
Given the current state $\centerset_t$, %suppose we have either $\ell \leq k$ or $(\ell-k)U_t \leq k \widehat{H}_t$. Then,
the expected uncovered cost after extra $t'$ rounds is
\begin{align*}
    \expect{U_{t+t'}(\pointset) \mid \centerset_t} \leq F_{t'}^\beta \rbr{\frac{U_t(\pointset)}{\HH_t(\pointset)}} \cdot \HH_t(\pointset).
\end{align*}
\end{lemma}

\begin{proof}
We prove this inequality by induction on the number of extra rounds. For $t'= 0$, since $F_0^\beta (x) = x$, the inequality holds.

Suppose the inequality holds for any $t'$ rounds, we show that this inequality is also true for $t'+1$ rounds. By the inductive hypothesis, we can get
$$
    \expect{U_{t+t'+1}(\pointset) \mid \centerset_{t+1}} \leq F_{t'}^\beta \rbr{\frac{U_{t+1}(\pointset)}{\HH_{t+1}(\pointset)}} \cdot \HH_{t+1}(\pointset).
$$
Taking expectation over the centers sampled at the round $t+1$, we  get
\begin{align*}
    \expect{U_{t+t'+1} \mid \centerset_t} \leq \E_{U_{t+1},\HH_{t+1}}\sbr{F_{t'}^\beta \rbr{\frac{U_{t+1}}{\HH_{t+1}}} \cdot \HH_{t+1} \mid \centerset_t}.
\end{align*}
In our thought experiment, we first draw the number of centers $Z_t(\cluster_i)$ for each cluster, then pick those centers independently. Suppose in the first stage the cost $\HH_t$ is not changed, while the uncovered cost $U_t$ decreases to $\UU_{t+1}$. In the second stage, $\HH_t$ changes to $\HH_{t+1}$ and $\UU_{t+1}$ decreases to $U_{t+1}$. Since two stages are independent, we can first take expectation over the randomness in the first stage. Since $F_{t'}^\beta$ is monotone and $U_{t+1} \leq \UU_{t+1}$, we have $F_{t'}^\beta(U_{t+1}/\HH_{t+1}) \leq F_{t'}^\beta(\UU_{t+1}/\HH_{t+1})$. By the concavity of $F_{t'}^\beta$ and Lemma~\ref{lem:uncovered}
\begin{align*}
    \expect{U_{t+t'+1} \mid \centerset_t} \leq \E_{\HH_{t+1}}\sbr{F_{t'}^\beta\rbr{\frac{F_1^\beta(U_t/\HH_t)\HH_t}{\HH_{t+1}}} \cdot \HH_{t+1} \mid \centerset_t}.
\end{align*}

Let $G_{t'}^\beta (x) = F_{t'}^\beta (\alpha/ x) x$ for constant $\alpha = F_1^\beta(U_t/\HH_t)\HH_t$. By Lemma~\ref{lem:Concave_Monotone_2} and Corollary~\ref{cor:5opt-martingale}, we can derive
\begin{align*}
    \expect{U_{t+t'+1} \mid \centerset_t} \leq \mathbb{E}_{\HH_{t+1}}\sbr{G_{t'}^\beta \rbr{\HH_{t+1}} \mid \centerset_t} \leq G_{t'}^\beta \rbr{\HH_t}.
\end{align*}
By Definition~\ref{def:recurrence}, we have
\begin{align*}
    \expect{U_{t+t'+1} \mid \centerset_t} \leq F_{t'}^\beta \rbr{F_1^\beta \rbr{\frac{U_t}{\HH_t}}}\HH_t = F_{t'+1}^\beta \rbr{\frac{U_t}{\HH_t}}\HH_t,
\end{align*}
which implies the inequality is true for $t+1$ rounds.
\end{proof}


\begin{theorem}~\label{thm:kpp_5}
For any $T > t >0$, the expected cost of $k$-means$\kpp$ algorithm is
$$
\expect{\cost_T(\pointset)} \leq F_{T-t}^\beta \rbr{1} \expect{\cost_t(\pointset)} + 5\opt_k(\pointset).
$$
\end{theorem}

\begin{proof}
By Lemma~\ref{lem:recursive} and Lemma~\ref{lem:Concave_Monotone}, we have
$$
\expect{U_{T} \mid C_t} \leq F_{T-t}^\beta \rbr{\frac{U_t}{\HH_t}} \HH_t \leq F_{T-t}^\beta \rbr{\frac{H_t + U_t}{\HH_t}} \HH_t.
$$
We consider two cases of the state $C_t$.
For the state $C_t$ with $U_t(\pointset) \geq \HH_t(\pointset) - H_t(\pointset)$, it holds that $H_t(\pointset) + U_t(\pointset) \geq \HH_t(\pointset)$. Let $G_{T-t}^\beta(x) = F_{T-t}^\beta(1/x)x$. By Lemma~\ref{lem:Concave_Monotone_2}, we have
$$
\expect{U_{T}(\pointset) \mid C_t} \leq F_{T-t}^\beta(1) \cdot(H_t(\pointset) + U_t(\pointset)).
$$
By Corollary~\ref{cor:5opt-martingale}, we can get $\expect{H_T \mid C_t} \leq \HH_t$. Combining it with the expected uncovered cost, we have
$$
\expect{\cost_T(\pointset) \mid C_t} \leq F_{T-t}^\beta(1)\cdot \cost_t(\pointset) +\HH_t.
$$
For the state $C_t$ with $U_t(\pointset) \leq \HH_t(\pointset) - H_t(\pointset)$, we have
$$
\expect{\cost_T(\pointset) \mid C_t} \leq \cost_t(\pointset) \leq U_t + \widehat{H}_t \leq \HH_t.
$$
Combining these two cases, we have for any state $C_t$
$$
\expect{\cost_T(\pointset) \mid C_t} \leq F_{T-t}^\beta(1)\cdot \cost_t(\pointset) +\HH_t.
$$
Therefore, taking expectation over $C_t$, we can derive
$$
\expect{\cost_T(\pointset)} \leq F_{T-t}^\beta(1) \expect{\cost_t(\pointset)} +5\opt_k(\pointset).
$$
\end{proof}

Note that $x_0 = 1$ satisfies the condition in Lemma~\ref{lem:F_decay} for any $\ell$. Thus, $F_{T-t}^\beta$ is upper bounded by $\frac{2}{\beta(T-t + t_0)}$ where $t_0=\ceil{2(1-\beta)/\beta}$. Therefore, combining Lemma~\ref{lem:F_decay}, Theorem~\ref{thm:kpp_main} and Theorem~\ref{thm:kpp_5}, we have the following corollary.%The expected cost of $k$-means\kpp will finally decrease to $5\opt_k(\pointset)$.

\begin{corollary}
Let $t_{\ell} = \log_{\gamma}(\opt_1(\pointset)/\opt_k(\pointset))$, where $\gamma = e^{-\ell/k}$ for $\ell\leq k$ and $\gamma = \sfrac{k}{e\ell}$ for $\ell \geq k$. The expected cost of the clustering returned by $k$-means$\kpp$ algorithm after $T \geq t_{\ell}$ rounds are
upper bounded as follows:

\noindent  For $\ell \leq k$,
$$
\expect{\cost_{T}(\total)} \leq \rbr{ \frac{2}{\beta(T-t_{\ell}+t_0)}\frac{6-e^{-\frac{\ell}{k}}}{1-e^{-\frac{\ell}{k}}} + 5}\opt_k(\pointset).
$$
\noindent For $\ell \geq k$,
$$
    \expect{\cost_{T}(\total)} \leq \rbr{ \frac{2}{\beta(T-t_{\ell}+t_0)}\frac{6-\sfrac{k}{e\ell}}{1-\sfrac{k}{e\ell}} + 5}\opt_k(\pointset),
$$
where $\beta = k(1-e^{-\ell/k})/\ell$ and $t_0 = \ceil{2(1-\beta)/\beta}$.
\end{corollary}
